# Supplementary material for: A Reduced Stochastic Model of Microservice Availability: Algorithms for Identification and Formal Analysis
Source: arXiv:2607.00740 source file (2026-10-22)
Supplement: Supplementary file 1 [file supplement-setup.tex]

% Include this file in the preamble of the article.
\RequirePackage{pdflscape}
\RequirePackage{geometry}
% Include supplement-body explicitly before \end{document} in main.tex.
% This keeps the appendix in the normal document flow and in the same PDF.
